# Supplementary material for: Forecasting Trajectory and Behavior of Road-Agents Using Spectral Clustering in Graph-LSTMs
Source: arXiv:1912.01118 source file (2020-08-05)
Supplement: Supplementary file 1 [file appendixA.tex]

\section{Data Preprocessing}
\label{sec: AppendixA}
We include all data and code used for data preprocessing with the supplementary material. Our data structure format (See Section~\ref{sec: dat_structures}) includes the time-stamp, road-agent ID, and the road-agent's spatial coordinates in the world coordinate frame. The process of obtaining these attributes, and utilizing them, to construct the data structures differs for all three datasets -- Lyft, Apolloscape, and Argoverse. We converted the three datasets to one unique representation that includes frame$\textunderscore$ID, road-agent$\textunderscore$ID, X, Y, dataset$\textunderscore$ID. 
% Sometimes, the terms frame$\textunderscore$ID, road-agent$\textunderscore$ID and dataset$\textunderscore$ID are interchangeably used with the terms  time$\textunderscore$stamp, agent$\textunderscore$ID and  scene$\textunderscore$ID respectively.
% Our approach in understanding each dataset based on the parameters above is described briefly below.

% \subsection{Level 5 Lyft dataset}
% % Understanding and extracting desired data from Level 5 Lyft dataset is a bit complex. 
% This dataset consists of 180 different traffic videos. Each video has a range of sample tokens (‘token’ here means a unique identifier assigned to each sample) with corresponding time stamps. For this range of time-stamps, we can obtain the camera data, lidar data and annotations of different road-agents. Within this range of time-stamps we are interested in the locations of the annotated road-agents and their unique identifiers (road-agent tokens). By understanding this data, we obtained and formatted the data into our desired representation.

% \subsection{ApolloScape Trajectory dataset}
% ApolloScape data is very straight-forward and provides the trajectory data in the format mentioned in \cite{ma2018trafficpredict}. The desired representation is extracted directly from the trajectory data provided.

% \subsection{Argoverse Motion Forecasting dataset}
% Argoverse Motion Forecasting data provides the locations of annotated road agents at each time-stamp. This data is directly extracted and had been formatted to our desired representation.

\subsection{Metadata}
To the best of our knowledge, there is very little known prior work using these datasets as they are relatively recent. As such, the raw datasets are not trivial to work with, due to their large size. In particular, to understand the performance, and gain interpretability, of an approach on a dataset, it is essential to study the underlying meta-features of each dataset. In Table~\ref{tab: meta}, we list some descriptive meta-features of the datasets. Additionally in this work, we also release code for efficient implementations for several key operations such as storage, extraction, querying, addition, and deletion on these datasets to facilitate future research using these datasets.

\begin{table}[h]
\centering
% \resizebox{.8\linewidth}{!}{%
\begin{tabular}{lcc} 
\toprule
Dataset & Batch & Avg. Density  \\
\hline

\multirow{3}{*}{Lyft} & Train & \Tstrut 0.80 \\
           & Val & 0.83 \\
           & Test & 0.84 \\                    
\midrule
\multirow{3}{*}{Argoverse} & Train & \Tstrut  0.75 \\
                           & Val & 0.67 \\
                           & Test & 1.67 \\

\midrule                           
\multirow{3}{*}{Apolloscape} & Train & \Tstrut  3.49 \\
                            & Val & 3.50 \\
                            & Test & 2.56 \\                         
            
% & Linear Regression                &&&&&&&& \\
% \cline{2-8}
% \midrule
% \toprule
%  \Tstrut &  \Bstrut & Overall \\
% \hline
% \multirow{3}{*}{Argoverse} & Guo et al~\cite{guo2019attention} & & & & & \\

% & Linear Regression                &&&&&&&& \\
% \cline{2-8}

% \midrule

% \hline
% \multirow{3}{*}{Argoverse} & Guo et al~\cite{guo2019attention} & & & & & \\

% & Linear Regression                &&&&&&&& \\
% \cline{2-8}
\bottomrule
\end{tabular}
% }
\caption{\textbf{Meta-Feature information} for the Lyft Level 5, Apolloscape, and the Argoverse datasets. The average density is reported by measuring the average number of road-agents per frame.}
\label{tab: meta}
% \vspace{-15pt}
\end{table}

% \begin{table*}[h!]
% \caption{Metadata for the Lyft Level 5, Apolloscape, and the Argoverse datasets.}
% \label{tab: accuracy}
% \centering
% \resizebox{.97\linewidth}{!}{%
% \begin{tabular}{lcccccccccccc}
% \toprule[1.1pt]
% \multirow{2}{*}{Dataset}                       &
% \multicolumn{3}{c}{Number of Videos\Tstrut }         &
% \multicolumn{3}{c}{Video Length \Tstrut }         &
% \multicolumn{3}{c}{Number of Vehicles\Tstrut }         &
% \multicolumn{3}{c}{Density \Tstrut }         & \\
% &
% mean \Tstrut & min & max \Bstrut &
% mean & min & max &
% mean & min & max &
% mean & min & max \\
% \midrule
% % \hhline{|=|=|=|=|=|=|=|=|=|=|=|=|=|=|=|}
% Lyft            &  1.163  &  1.242  &  4.423  &  8.640  & 5.031  &  9.882   &  6.66  &  11.27  & 0.262  &  0.270  &  0.010  &  0.01  \\ 
% Argoverse       &  0.871  &  0.884  &  0.635  &  3.091  & 1.039  &  3.079   &  0.930   &  1.850  & 0.244  & 0.243  &  0.005  &  0.005  \\ 
% Apolloscape     &  0.013  &  0.017  &  1.248  &  11.240  & 1.283  &  11.674  &  0.110  &  0.150  & 0.011  &  0.007  &  -  &  - \\ 
% \bottomrule[1.1pt]
% \end{tabular}
% }
% \vspace{-10pt}
% \end{table*}

% in Argoverse, we have much more videos than in Lyft and Apolloscape; in Apolloscape, the number of video is small while its length is long and various; vehicle density is much higher in Apolloscape than other datasets.
\begin{figure}[t]
    % \vspace{-20pt}
    \includegraphics[width=\columnwidth]{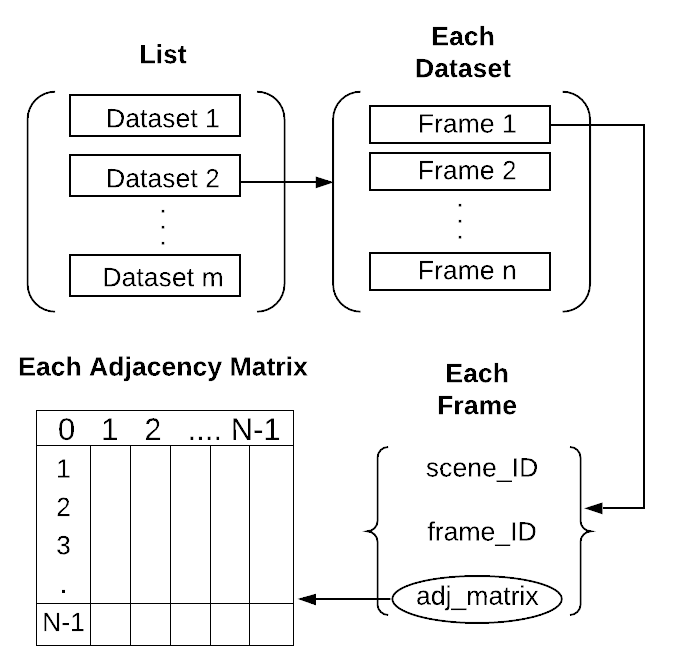}
    \caption{\textbf{Schematic:} Data structure for Adjacency matrices.}
    % \vspace{-10pt}
    \label{fig:adjacency}
\end{figure}
\section{Data Structures}
\label{sec: dat_structures}
This section describes the different data structures that are used in our approach. The implementations of these data structures are included with the code. 

\subsection{Adjacency Matrices}
Figure~\ref{fig:adjacency} shows a schematic for the data structure used to create the adjacency matrices for the whole dataset. The adjacency matrix corresponding to a traffic graph captures the interactions between all agents within that frame. A python list is used to store adjacency data of each traffic video, where each video is again a list of all frames in that dataset. Each frame is a python dictionary containing the `dataset$\textunderscore$ID', `frame$\textunderscore$ID' and `adj$\textunderscore$matrix'. Each adjacency matrix is an array of size $ N \times N$, where $N$ is the total number of agents in the dataset. The adjacency matrices are used to form the Laplacian matrices that are updated at every time-step according to equation $3$.

\subsection{Input for Stream 1}
Figure \ref{fig:stream1} shows the schematic for the data structure used to prepare the input for stream 1. The implementation consists of a python list of dictionaries. Each dictionary denoted as item$\textunderscore$1, item$\textunderscore$2....item$\textunderscore$n in Figure~\ref{fig:stream1}, has three keys- 'dataset$\textunderscore$ID', 'agent$\textunderscore$ID', and 'sequence'. The value of the 'sequence' consists of an array of size $n \times 2$, where $n$ is the length of either the observation sequence or prediction sequence. Each row of this sequence array consists of the global $X,Y$ coordinates, respectively, of the road-agent at that observation or prediction time step.  

\begin{figure}[h]
    \includegraphics[width=\columnwidth]{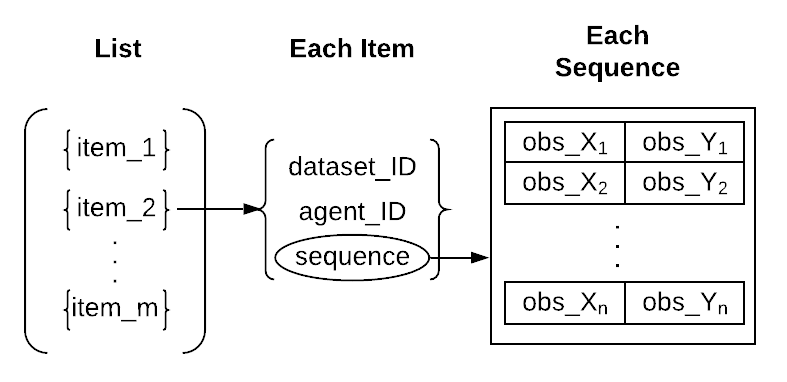}
    \caption{\textbf{Schematic:} Data structure for the input to Stream1.}
    % \vspace{-10pt}
    \label{fig:stream1}
\end{figure}

\subsection{Input for Stream 2}
Figure~\ref{fig:stream2} shows the schematic for the data structure used to prepare the input for stream 2. This data structure is similar to the stream1 data structure in that it also consists of  a list of dictionaries. Each dictionary has the keys `dataset$\textunderscore$ID', `agent$\textunderscore$ID', `mean$\textunderscore$theta$\textunderscore$hat', `mean$\textunderscore$theta', and $F_1,F_{2}, \ldots, F_{n}$, where $n$ is the length of the observation sequence or prediction sequence, respectively. Each $F_i$ represents the $i^{\textrm{th}}$ frame which is an array of size $2 \times N$, where $N$ denotes the total number of road-agents in that traffic video. The columns of this array stores the global $X,Y$ coordinates of all the road-agents at $i^{\textrm{th}}$ frame. The keys, `mean$\textunderscore$theta$\textunderscore$hat' and `mean$\textunderscore$theta' store information corresponding to the ground-truth behavior labels for that sequence of frames.

\begin{figure}[h]
    % \vspace{-5pt}
    \includegraphics[width=\columnwidth]{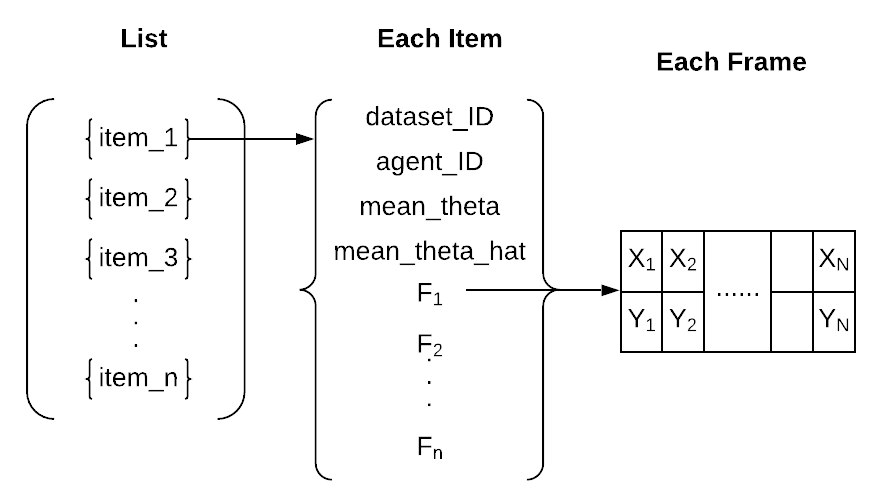}
    \caption{\textbf{Schematic:} Data structure for the input to Stream2.}
    % \vspace{-5pt}
    \label{fig:stream2}
\end{figure}

% Further details on data pre-processing and metadata extraction can be found in Appendix~\ref{sec: AppendixA}.
