# Supplementary material for: Forecasting Trajectory and Behavior of Road-Agents Using Spectral Clustering in Graph-LSTMs
Source: arXiv:1912.01118 source file (2020-08-05)
Supplement: Supplementary file 2 [file appendixB.tex]

\section{Motivation for Equation 3}

Our intuition is that a road-agent should remember the interactions with not just its current neighbors, but all neighbors it has observed up until current time $t$. Therefore, the first term on the RHS stores the information of road-agents uptil time $t$, while the second term on the RHS contains the information of the newly observed road-agents at time $t+1$.

% \section{Computing $\Lambda$ in the Behavior Prediction Algorithm}

\section{Analysis of Stream 2 Continued}

In Section 4.2, we presented a behavior prediction algorithm that begins by forming the set of predicted spectrums from the second stream, $\mc{U}= \{ U_{T+1}, U_{T+2}, \dots, U_{t+\tau} \}$. The success of the algorithm depends on the accuracy of these predictions, that further depends on the amount of correlation existing between the sequence of eigenvectors. In Section 4.3, we proved an upper bound for the error distance between the $j^{\textrm{th}}$ eigenvectors of $L_t$ and $L_{t+1}$, denoted as $\phi_j$. We showed that $\phi_j = \bigO{\sqrt{n} \delta_{max}}$, where $\delta_{max}$ is the maximum component of $\delta_t$.

An alternative approach to computing the spectrums $\{U_{T+1}, \ldots, U_{T+\tau}\}$ is to first form traffic-graphs from the predicted trajectory given as the output from the stream 1. Next, obtain the corresponding Laplacian matrices for these traffic-graphs. Finally, use standard eigenvalue algorithms to compute the spectrum sequence. This is, however, a relatively sub-optimal approach as in this case, $\phi = \bigO{n L_{max}}$, with $L_{max} \gg \delta_{max}$.

\section{Additional Related Work}

In Section 6, we compared our approach against several prominent SOTA deep learning-based trajectory prediction algorithms. However, it is worth noting that there are other additional methods in the trajectory prediction literature that we have not considered in this present work. Social-LSTM~\cite{social-lstm} is a popular approach for trajectory prediction of pedestrians in crowds. However, in the interest of clarity, we provide here an explanation regarding its exclusion from the experimental setup:

\begin{itemize}
    \item The official implementation of Social-LSTM has been recently withdrawn from public access. Therefore, any results obtained via custom implementations would not offer an unbiased view of the method compared to prior works, that have used the official implementation before its removal.
    
    \item Instead of presenting a somewhat biased comparisons with a well-known pedestrian trajectory prediction method, we compare with CS-LSTM~\cite{nachiket}, which is a slight modification of the Social-LSTM method for road-agent trajectory prediction.
\end{itemize}

\section{Training Details of Comparison Methods}

\begin{itemize}
    \item \textbf{TraPHic \& CS-LSTM}: Implementations of both methods can be found in \cite{chandra2019robusttp}. On the Lyft, Argoverse, and Apolloscape datasets, we use NLL loss and MSE loss for pretraining and training. We perform a hyperparameter grid search with 10-40 epochs of batch size $64$ and $128$. We use the adam, adamax, Rprop, and RMSprop optimizers, with learning rates of $0.01$, $0.001$, and $0.005$, respectively, and dropouts between $0.4-0.6$. In TraPHic, we get the best result on Lyft and Argoverse with the adamax optimizer with a dropout of $0.4$ and $0.5$, respectively, and on Apolloscape with the adam optimizer with a dropout of $0.5$. In CS-LSTM, our best result on Lyft is obtained with the adamax optimizer with a dropout of $0.4$, and on Argoverse and Apolloscape with the adam optimizer with a dropout of $0.5$. However, compared to other methods, these two methods perform poorly as time increases.
    
    \item \textbf{Social-GAN}: We use the standard implementation in~\cite{social-gan}. On each of the three datasets, our hyperparameter grid search ranges from $1500-3000$ epochs of batch size $32$, using adam, adamax, Rprop, and RMSprop optimizers, with a learning rate of $0.001$, $0.0001$ and $0.0005$, respectively, on both generator and discriminator. We achieve the best result with the adamax optimizer on Lyft and Argoverse, and adam optimizer on Apolloscape, all with a learning rate of $0.0005$. Due to limited GPU memory, we were not able to experiment on larger batch sizes. Since Social-GAN is a pedestrian trajectory prediction approach, we scaled down the trajectories in all three datasets by a factor of $20$ to resemble the trajectories of pedestrians. Even so, we achieve unstable results during testing.

    \item \textbf{Enc-Dec}: We implement this method from scratch, similar to the implementation of stream 1 in our two-stream network. The key difference is that we train Enc-Dec with the MSE loss whereas we train our two stream network with the NLL loss function. We obtain optimum results for Enc-Dec after $50$ epochs with batch size of $40$ and learning rate of $0.001$.

    \item \textbf{GRIP}: We also implement this method following the approach in~\cite{li2019grip}. We obtain the best results with batch size of $128$ and learning rate of $0.001$. 
    % Due to limited time and computational resources, we only train on this model several batches and got our results on testing set.
\end{itemize}

\subsection{Training Details}
\label{subsec: implementation}
We use 2 Nvidia GeForce RTX 2080 Ti GPUs with 12GB memory each, for all experiments. Initially, we trained both streams together for 20 epochs. However, we found that by training stream one first for 20 epochs, and then training both streams for another five epochs generated the best results, reported in Table~\ref{tab: accuracy}.

Due to the computations involved in obtaining the Laplacian matrices and their corresponding eigenvectors, data processing for stream two is both time-consuming and expensive in terms of computational resources. Consequently, we choose $6310$, $5126$, and $5073$ valid trajectories to form the training set, and $769$, $1678$ and $1012$ valid trajectories to form the testing set for the Lyft, Argoverse and Apolloscape datasets, respectively. We consider the trajectory for a road-agent to be valid if that road-agent is present for at least 8 seconds (3 observation + 5 prediction ) in Lyft and Apolloscape. In Argoverse, we only use the first 2 seconds as an observed trajectory to predict the next 3 seconds since each video in Argoverse is limited to 5 seconds. 

\textbf{Stream 1: }The input to stream one consists of trajectory tensors of size $B\times T \times 2$, with $B=128$ representing the batch size, $T=3$ seconds denoting the length of the observed trajectory, and 2-dimensional spatial coordinates. In stream 1, our training converges in 20 epochs in approximately 20 minutes for each data set. The best results from stream one are obtained by using the RMSprop optimizer~\cite{rmsprop} with a learning rate of $0.001$.

\textbf{Stream 2: }The input to stream 2 consists of a sequence of eigenvectors represented as a tensor of size $k \times B \times T \times N$, where $k$ denotes the number of eigenvectors for each Laplacian matrix, $N$ is the number of road-agents in the traffic-video. It takes approximately 42 hours per epoch to process the data for stream 2. Therefore, we pre-compute the input data for stream two offline, which reduces the training time to 2.2, 1.5, and 1.2 hours per epoch for Lyft, Argoverse, and Apolloscape, respectively. The hyper-parameters for stream 2 are identical to those used in stream 1.
\vspace{-5pt}
